# Supplementary material for: LLM-Rec: Personalized Recommendation via Prompting Large Language Models
Source: arXiv:2307.15780 source file (2024-04-02)
Supplement: Supplementary file 1 [file appendix_KAR_All_Beauty.tex]

\begin{table*}[h]
    \caption{Response generated by {\sc ChatGPT} about the question \textit{``List the importance factors or features that determine whether a user will be interested in a product of the All Beauty category.''} }
    \centering
    \small
    \adjustbox{max width=\textwidth}{
    \begin{tabular}{p{\textwidth}}
        \toprule[1.1pt]

        The interest of users in products within the "All Beauty" category can be influenced by a variety of factors or features. Here's a list of some of the key importance factors:

Quality and Effectiveness: The product's ability to deliver on its promises, such as improving skin health, enhancing beauty, or resolving specific beauty concerns.

Ingredient Safety: Consumers often look for products with safe, non-toxic ingredients, especially those who have sensitive skin or are environmentally conscious.

Brand Reputation: A well-known and trusted brand can significantly influence a buyer's decision, as it often assures quality and reliability.

Price and Value for Money: The product should be competitively priced and offer good value for the quality and quantity provided.

Packaging and Aesthetics: Attractive and functional packaging can greatly enhance the appeal of beauty products.

Product Range and Variety: A wide range of options to cater to different skin types, beauty needs, and preferences can attract a broader audience.

Customer Reviews and Ratings: Positive feedback and high ratings from other users can significantly impact a potential buyer's decision.

Ethical Considerations: This includes cruelty-free, vegan, eco-friendly, and sustainable practices, which are increasingly important to many consumers.

Innovativeness: Products that offer new, unique, or advanced features or formulations can stand out in a crowded market.

Availability and Accessibility: Easy availability, both online and in physical stores, as well as international shipping options, can influence interest.

Marketing and Promotion: Effective advertising, influencer endorsements, and promotional offers can draw attention to the product.

Regulatory Compliance: Adherence to health and safety standards and regulations enhances trustworthiness.

Sensory Experience: The texture, fragrance, and overall feel of the product during use can be a significant factor.

Cultural and Trend Alignment: Products that align with current beauty trends or cultural preferences tend to be more popular.

Each of these factors can play a crucial role in determining a user's interest in a beauty product, and their relative importance can vary depending on the specific target market and consumer demographics.\\

        \bottomrule[1.1pt]
    \end{tabular}}
    \label{tab:appendix_KAR_all_beauty}
\end{table*}
