# Supplementary material for: LLM-Rec: Personalized Recommendation via Prompting Large Language Models
Source: arXiv:2307.15780 source file (2024-04-02)
Supplement: Supplementary file 2 [file appendix_KAR_Appliances.tex]

\begin{table*}[h]
    \caption{Response generated by {\sc ChatGPT} about the question \textit{``List the importance factors or features that determine whether a user will be interested in a product of the Appliances category.''} }
    \centering
    \small
    \adjustbox{max width=\textwidth}{
    \begin{tabular}{p{\textwidth}}
        \toprule[1.1pt]

        The interest of users in products within the "Appliances" category can be influenced by several key factors or features. Here's a list of some of the most important ones:

Functionality and Performance: The primary concern is how well the appliance performs its intended function, such as the efficiency of a refrigerator in cooling or a washing machine in cleaning clothes.

Durability and Reliability: Consumers often look for appliances that are durable and reliable, with a long lifespan and minimal need for repairs.

Energy Efficiency: Appliances that are energy-efficient and cost-effective to operate can be more appealing, especially with rising energy costs.

Brand Reputation: A well-known and trusted brand can be a significant deciding factor, as it often implies quality and reliability.

Price and Value for Money: Competitive pricing and good value for the quality and features offered are important considerations.

Design and Aesthetics: The appearance of the appliance, including its size, shape, and color, and how well it fits with the user's home décor and space constraints.

Innovative Features: Advanced or unique features that set the appliance apart from others in the market can be a major draw.

User-Friendly Interface: Ease of use, including simple controls and intuitive interfaces, can make an appliance more appealing.

Customer Reviews and Ratings: Positive feedback and high ratings from other users can significantly influence a potential buyer's decision.

Warranty and Customer Support: A good warranty and responsive customer support can increase the attractiveness of an appliance.

Safety Features: Built-in safety features that prevent accidents and injuries are crucial for many consumers.

Noise Level: Particularly for appliances used frequently, like dishwashers or washing machines, a lower noise level can be a desirable feature.

Smart Technology Integration: The ability to connect and interact with smart home systems or smartphones for added convenience.

Availability and Accessibility: Easy availability in stores or online, as well as convenient delivery and installation options.

Environmental Impact: Eco-friendly appliances that have a lower environmental impact can be more appealing to environmentally conscious consumers.

Each of these factors plays a crucial role in influencing a user's interest in an appliance product, and their relative importance can vary depending on the specific needs, preferences, and budget of the consumer.\\

        \bottomrule[1.1pt]
    \end{tabular}}
    \label{tab:appendix_KAR_appliances}
\end{table*}
