# Supplementary material for: LLM-Rec: Personalized Recommendation via Prompting Large Language Models
Source: arXiv:2307.15780 source file (2024-04-02)
Supplement: Supplementary file 3 [file appendix_KAR_Automotive.tex]

\begin{table*}[h]
    \caption{Response generated by {\sc ChatGPT} about the question \textit{``List the importance factors or features that determine whether a user will be interested in a product of the Automotive category.''} }
    \centering
    \small
    \adjustbox{max width=\textwidth}{
    \begin{tabular}{p{\textwidth}}
        \toprule[1.1pt]

        Interest in products within the "Automotive" category is influenced by a range of factors and features. These are essential considerations for consumers when selecting automotive products, such as cars, parts, accessories, or services:

Performance and Reliability: The ability of the vehicle or part to perform as expected over time, including engine efficiency, speed, handling, and reliability in various conditions.

Safety Features: Key safety features like airbags, anti-lock braking systems (ABS), traction control, and advanced driver assistance systems (ADAS) are crucial for consumer confidence.

Fuel Efficiency and Emissions: Fuel economy and low emissions are increasingly important for cost-saving and environmental reasons.

Brand Reputation and History: The reputation of the manufacturer or brand for quality, reliability, and customer satisfaction plays a significant role.

Price and Value for Money: The cost of the vehicle or product relative to its features and compared to competitors.

Design and Aesthetics: The visual appeal of a vehicle or accessory, including style, color, and overall design.

Comfort and Interior Features: The comfort of the seats, interior space, climate control, infotainment systems, and other interior features.

Technological Innovations: Advanced technology features like touchscreen displays, connectivity options, navigation systems, and autonomous driving capabilities.

Maintenance Costs and Serviceability: The ease and cost of maintaining and servicing the vehicle or product over its lifespan.

Warranty and After-Sales Service: The length and coverage of the warranty, as well as the quality of after-sales service and support.

Customer Reviews and Ratings: Feedback and experiences of other users with the product or service.

Resale Value: The expected depreciation and resale value of the vehicle or product.

Environmental Impact: For many consumers, the ecological footprint of the vehicle, including the use of sustainable materials and production methods, is important.

Compatibility and Integration: For automotive parts and accessories, compatibility with the vehicle and ease of integration are key.

Availability and Accessibility: The ease of purchasing the vehicle or product, including availability at local dealerships or stores, and online availability.

These factors collectively influence a consumer's interest and decision-making process in the automotive category. The weightage of each factor can vary significantly based on individual preferences, needs, and the specific type of automotive product being considered.\\

        \bottomrule[1.1pt]
    \end{tabular}}
    \label{tab:appendix_KAR_automotive}
\end{table*}
